# Supplementary material for: Arrow Matrix Decomposition: A Novel Approach for Communication-Efficient Sparse Matrix Multiplication
Source: arXiv:2402.19364 source file (2024-03-20)
Supplement: Supplementary file 1 [file appendix.tex]

\section{Additional Proofs}

\subsection{Linear arrangement}

%Note that this result immediately implies an $\Omega(n\Delta)$ lower bound on the linear arrangement of bounded treewidth graphs and $K_r$ minor-free graphs (as trees are in both families of graphs).

%\todos{Can we get a more general bound that relates the existence of MLA to the existence separators? I.e., if we have an mla of cost $ns\Delta$, we can find a separator of size $O(s)$?}

We show in Section \ref{sec:tree-arrow-decomposition} how we can get a  $O(\Delta)$-arrow compact matrix decomposition for trees, which is an $O(\log n)$ factor better than what we would get using \textsc{Separator-LA}.

%We show next that we can improve the bounds on the decomposition for trees by a $\log n$ factor using an approach that does not make use of the cost of the linear arrangement.

\subsubsection{Clique minor free graphs}

Efficient constructions for small separators were initially shown in planar graphs~\cite{doi:10.1137/0136016}. Kawarabayashi and Reed~\cite{DBLP:conf/focs/KawarabayashiR10} generalized these results to families of graphs that exclude some clique as a so-called \emph{minor}:
A graph $H$ with vertices $h_1, \dotsc, h_r$ is a \emph{minor} of $G$ if and only if there are disjoint sets of vertices $A_1, \dotsc, A_r$ in $G$ such that for each edge between a pair of vertices $h_i$ and $h_j$, there is an edge between a vertex in $A_i$ and a vertex in $A_j$. A graph is $H$-minor free if $H$ is not a minor of $G$.

\begin{theorem}[Kawarabayashi and Reed~\cite{DBLP:conf/focs/KawarabayashiR10}]
	A $K_r$-minor free graph has a $\frac{2}{3}$-separator of size $O(r \sqrt{n})$.
\end{theorem}
This result generalizes previous results on planar and bounded genus graphs. One disadvantage of this approach is that its running time is super-exponential in $r$ (but it is nearly-linear in $n$).
We conclude by Lemma \ref{lem:mla-separator}:
\begin{corollary}
A $K_r$-minor free graph has a linear arrangement of cost $O(n^{\frac{3}{2}} \Delta r)$.
\end{corollary}
%\begin{proof}
%Follows from a refinement of \Cref{lem:mla-separator}: Observe that when the $\frac{2}{3}-$separators of a subgraph of size $n$ have size $\omega(1)$, the cost decreases geometrically with the recursion depth and resolves to $O(n\Delta s(G))$.
%\end{proof}

%
As planar graphs are $K_5$-minor free~\cite{bondy2011graph}, we get linear arrangements of cost $O(n^{\frac{3}{2}}\Delta)$.

%a $c$-compacting $O(\sqrt{n} \Delta c)$-arrow matrix decomposition for such graphs. % In particular, we can compute nontrivial arrow decompositions of order $O(1)$ for such graphs.

If we exclude only so-called shallow minors, we can find good separators in an even bigger family of graphs:
A graph $H$ with vertices $h_1, \dotsc, h_r$ is a \emph{depth} $l$ \emph{minor} of $G$ if and only if there is a disjoint set of vertices $A_1, \dotsc, A_r$ in $G$ where $G[A_i]$ has diameter at most $l$ and for each edge between a pair of vertices $h_i$ and $h_j$, there is an edge between $A_i$ and $A_j$.
There are efficiently computable small separators in graphs with no $K_r$-minor of low depth:
\begin{theorem}[Plotkin, Rao, and Smith~\cite{DBLP:conf/soda/PlotkinRS94}]
	A graph $G$ with no $K_r$-minor of depth $l$ has a $\frac{2}{3}$-separator of size $O(\frac{n}{l} + l r^2 \log n )$. It can be computed in $O(\frac{mn}{l})$ work.
\end{theorem}
An advantage of this algorithm is that its running time does not deterioriate with $r$ and it is fairly simple, mainly relying on graph traversals and set intersections. Note that by setting $l=\frac{\sqrt{n}}{t\sqrt{\log n}}$ we get a $\frac{2}{3}$-separator of size $O(r\sqrt{n \log n})$ in any $K_r$-minor free graph. 

\begin{corollary}
A graph with no $K_r$-minor of depth $l$ has a linear arrangement of cost $O(n \Delta (\frac{n}{l} + l r^2 \log n))$.
\end{corollary}

%A graph that excludes $K_r$ as a minor has a $O(\sqrt{n}r)$-sized $\frac{2}{3}$-separator that can be computed in polynomial time~\cite{DBLP:conf/focs/KawarabayashiR10}. For $K_r$-minor free graphs we can construct an arrow matrix decomposition using their separators. 

\subsubsection{Bounded Treewidth Graphs}

Another family of graphs with small separation number are bounded \emph{treewidth} graphs. Specifically, graphs with treewidth $\tau$ have separation number $\tau+1$~\cite{DBLP:journals/ejc/BottcherPTW10, ROBERTSON1986115}. Graphs that have bounded treewidth include series parallel graphs ($\tau=2$) and low-diameter planar graphs. Specifically, a planar graph has treewidth at most $3D(G)-2$ \cite{DBLP:journals/jgaa/Eppstein99}. Observe that we have the reverse situation for planar graphs compared to the (maximum) bandwidth problem: For an arrow matrix decomposition, planar graphs of low diameter have a low bandwidth matrix decomposition, whereas those graphs have a large bandwidth.

\begin{corollary}
A graph with treewidth $\tau$ has a linear arrangement of cost $O(n\Delta \tau \log n)$.
\end{corollary}

\subsection{Spmm IO bounds}
%In this section, we show

\minisec{Direct 1D decomposition} The 1D algorithm computes the rows of the result matrix one after the other~\cite{TODO}. This requires moving the whole matrix \mat{X} into internal memory for \emph{each} row of the result. This requires a \emph{quadratic} number of IO's in the number of rows as there is almost no temporal locality. % Specifically, if $M \in o(nk)$ and $M \geq 2k$ the 1D algorithm takes at least $n*\ceil{\frac{nk}{B}} + \ceil{\frac{\nnz{\mat{A}}}{B}}$ IO's in the worst case.

\begin{lemma}
Consider the  matrices $\mat{A}\in R^{n\times n} $ and $\mat{X} \in R^{n\times k}$. If $2k\leq M \leq \frac{nk}{2}$, The 1D algorithm for computing $\mat{A}\mat{X}$ takes at least $n*\ceil{\frac{nk}{2B}} + \ceil{\frac{\nnz{\mat{A}}}{B}}$ IO's and at most $n*\ceil{\frac{nk}{B}} + \ceil{\frac{\nnz{\mat{A}}}{B}}$ IO's in the worst case.
\end{lemma}
\begin{proof}
TODO
\end{proof}

\minisec{Direct 2D decomposition} The 2D algorithm slices the matrix \mat{A} into tiles (splitting it both by row and column). Each result tile is computed as the reduction of multiplying one row of tiles of \mat{A} with \mat{X}. This results in some data reuse within the tiles. If $k\leq \sqrt{M}$, the tiles of $A$ can be chosen as $\Theta(\sqrt{M})\times \sqrt{M}$ and the tiles of \mat{X} and \mat{C} as $\sqrt{M}\times k$ \lukas{TODO: check optimal size of tiles}

\begin{lemma}
Consider the  matrices $\mat{A}\in R^{n\times n} $ and $\mat{X} \in R^{n\times k}$. If $\sqrt{M}\geq k$, the 2D algorithm for computing $\mat{A}\mat{X}$ takes \lukas{TODO} IO's in the worst case.
\end{lemma}
\begin{proof}
TODO
\end{proof}
